# Supplementary material for: Metrology of time-domain soft X-ray attosecond pulses and re-evaluation of pulse durations of three recent experiments
Source: arXiv:1905.09526 source file (2019-05-23)
Supplement: Supplementary file 1 [file Supplement_Material_XZ0424.pdf]

# Supplementary material for Metrology of time-domain soft X-ray attosecond pulses and re-evaluation of pulse durations of three recent experiments

Xi Zhao[1], Su-Ju Wang[1], Wei-Wei Yu[1,2], Hui Wei[1], and C. D. Lin[1]
[1] *Department of Physics, Kansas State University, Manhattan, KS 66506, USA*
[2] *School of Physics and Electronic Technology, Liaoning Normal University, Dalian 116029, People's Republic of China*

PACS numbers: 32.80.Rm, 42.50.Hz, 42.65.Ky

## I. SENSITIVITY OF THE AC PATTERN TO ATTOCHIRP ON THE WAVELENGTH AND INTENSITY OF THE IR LASER FIELD

The sensitivity of the AC pattern to attochirp (only linear chirp is considered in this section) on the wavelength and intensity of the IR laser field is illustrated in Fig. S1 (a) and (b). We define a parameter $\gamma$, which is the ratio of the duration of the chirped pulse to the duration of the transform-limited pulse (20 as in this case), to indicate the amount of attochirp. The change of the metric volume from the autocorrelation (AC) pattern as a function of $\gamma$, i.e. the slope in Fig. S1, would reflect how easily the SXR or XUV pulses can be retrieved. A larger slope means a better sensitivity to the spectral phase, which leads to a faster convergence and a better performance of the phase retrieval process. Ideally one would like to choose intensity and wavelength of the streaking laser field that give steeper slopes in Figs. S1 (a) and (b) if possible.

The laser parameters used in Fig. S1 are the same as those in Fig. 1 of the main text except for the IR intensities and wavelengths. In Fig. S1 (a), we fix the IR intensity to $2.5 \times 10^{12}$ W/cm$^2$ and vary its wavelength. The metric volume decreases monotonically with $\gamma$ in all cases. Based on our calculations for three different wavelengths, the best sensitivity is achieved at 800 nm, while the performance becomes lower when we either increase the wavelength to 1800 nm or decrease the wavelength to 400 nm.

In Fig. S1 (b), we plot the dependence of the metric volume from the AC pattern as a function of $\gamma$ for various IR intensities at the fixed IR wavelength 1800 nm. It is shown that the slope decreases with decreasing IR intensity, which indicates that the streaking contrast is weaker at a lower IR intensity and makes the retrieval method less sensitive to the spectral phase. This would imply that the low IR intensity required for the PROOF method is less favorable.

## II. EFFECT OF MULTIPLE PHOTOIONIZATION CHANNELS

In Fig. 3 of the main text, our PROBP-AC method accounts for photoelectrons ejected from the $5p$, $5s$, and $4d$ subshells of Xe. It is noted that in Gauminitz et al Ref.[1], only 5p and 5s electrons are included. Fig. S2 shows the yields of photoelectrons, which is given by the product of dipole intensity and the XUV intensity $|d(E)|^2 |E_{XUV}(E)|^2$, for each of the three channels. The dipole data and the XUV intensity, as functions of the photoelectron energy $E$, are identical to those used in Ref.[1]. Note that from 40 to 60 eV, the dominant contribution to the photoelectron spectra is from the $4d$ channel. In the range from 60 to 75 eV, both $5p$ and $5s$ channels have significant contributions to the spectra. The $4d$ channel becomes insignificant for electron energy above 63 eV. Above 75 eV, the $5p$ channel becomes the dominant channel. As the energy is above 80 eV, the intensity of the $5p$ channel is at least one order of magnitude larger than those from the $5s$ and $4d$ channels.

Fig. S3(a) shows the retrieved spectral phase and Fig. S3(b) shows the retrieved intensity of the XUV in the time domain, by including only 5p, and only 5s and 5p, respectively, and are compared to results including all three channels. By including all three channels we obtained pulse duration of 62 as. By including only one or two channels, the retrieved pulses are 74 and 72 as, respectively. For comparison, in Ref.[1], only the 5p and 5s channels were included and they retrieved a pulse duration of 43 as.

## III. DEPENDENCE OF PHASE RETRIEVAL FROM DIFFERENT BLOCKS

The PROBP-AC methods can retrieve the pulses from just one block of the AC, or from a few blocks. By covering the spectrograms over a few MIR optical cycles may in principle average over the noises in the signals. However, this procedure is preferred only if the noises are completely random. In the main text, by analyzing the spectrogram in Fig. 2(a), we noted that the spectrogram taken before $\tau = 1$ fs appears to be better behaved. Thus, we chose block 5 to retrieve the XUV and the MIR pulses, to obtain the results shown in Figs. 3(d-f). Indeed, the spectrogram in Fig. 2(a) was found to have 30%-40% higher signals in the region near $(E,\tau)$=(75 eV, 2 fs). Such singular behavior is not expected in the spectrogram and it is likely due to noises. Thus, phase retrieval including data from this region is less desirable. To elaborate this point, we note that blocks 1 and 2 (which is equivalent to 4) contain data from this undesirable re-

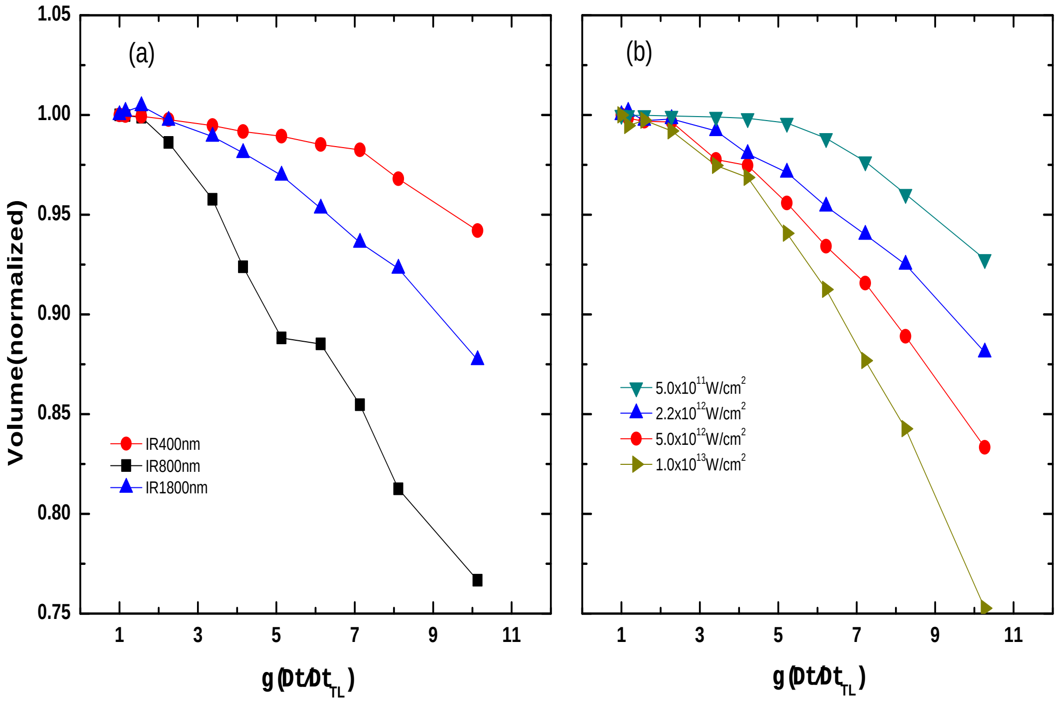


FIG. S1: (Color online) The normalized volume of the autocorrelation pattern as a function of $\gamma$, which is the pulse duration ratio between the linearly chirped pulse and the TL one. In (a), the IR intensity is fixed at $2.5 \times 10^{12}$ W/cm$^2$ and the IR wavelengths are chosen to be 400 nm, 800 nm, and 1800 nm. In (b), the IR wavelength is fixed at 1800 nm and four intensities are used.

gion, while blocks 3, 5 (equivalent to 7), and 6 do not contain those data. We use the same retrieval method and dipole parameters as we use in analyzing block 5 to analyze block 1, 2, 3 and 6. The results are shown in Figs. S4 and S5. In Fig. S4, on the top row, the ACs of each block obtained from the experiment of Ref.[1] are compared to the ACs generated from our retrieved pulses, shown in the bottom row, respectively. Clearly, one can see that they exhibit very good overall agreement for each pair. In Fig. S5(a), the spectral phases retrieved from blocks 1 and 2 are very close to each other, but they are very different from the ones retrieved from blocks 3 and 6. We note that the latter are in good agreement with the one reported in Fig.3(e) retrieved from block 5. In fact, from blocks 3, and 6, we retrieved pulse durations of 61 as and 60 as, respectively, which are very close to the 62 as retrieved from block 5. In contrast, from blocks 1 and 2, we retrieved pulse durations of 90 as, and 80 as, respectively. The intensity profile in the time domain for the five retrieved pulses are shown in Fig. S5(b). Results from blocks 1 and 2 are quite different from blocks 3,5, and 6. Based on these results, we would suggest that the "noise" in the spectrogram near ($E$,$\tau$)=(75 eV, 2 fs) in Ref.[1] contributes to this difference. We also note that pulse duration alone is not a good representation of the temporal behavior of the SXR attosecond pulses since the intensity profile can still differ significantly, see the intensity profile obtained from block 3 as compared to those from blocks 5 and 6 in Fig. S5(b).

## IV. COMPARISON OF MERITS

To compare the difference between the experimental and retrieval results, we define the merit by:

$$\varepsilon_f = \frac{\sum_{i=1}^{M}\sum_{j=1}^{N}\left|f_{\text{output}}(i,j) - f_{\text{exp}}(i,j)\right|^2}{\sum_{i=1}^{M}\sum_{j=1}^{N}\left|f_{\text{exp}}(i,j)\right|^2}, \qquad \text{(S1)}$$

where $f_{\text{output}}(i,j)$ is the two dimensional output from the retrieval, $f_{\text{exp}}(i,j)$ is the experimental data, $M$ and $N$ are the number of grid points on the time delay and the photoelectron energy, respectively. The function $f$ could be the streaking trace (S) or the AC pattern. Before making any comparison, we normalize streaking traces and AC patterns with respect to their maximum values such that they have values between 0 to 1. If the retrieval results $f_{\text{output}}(i,j)$ match perfectly with the experimental data $f_{\text{exp}}(i,j)$, then the merit $\varepsilon_f = 0$. We calculate the

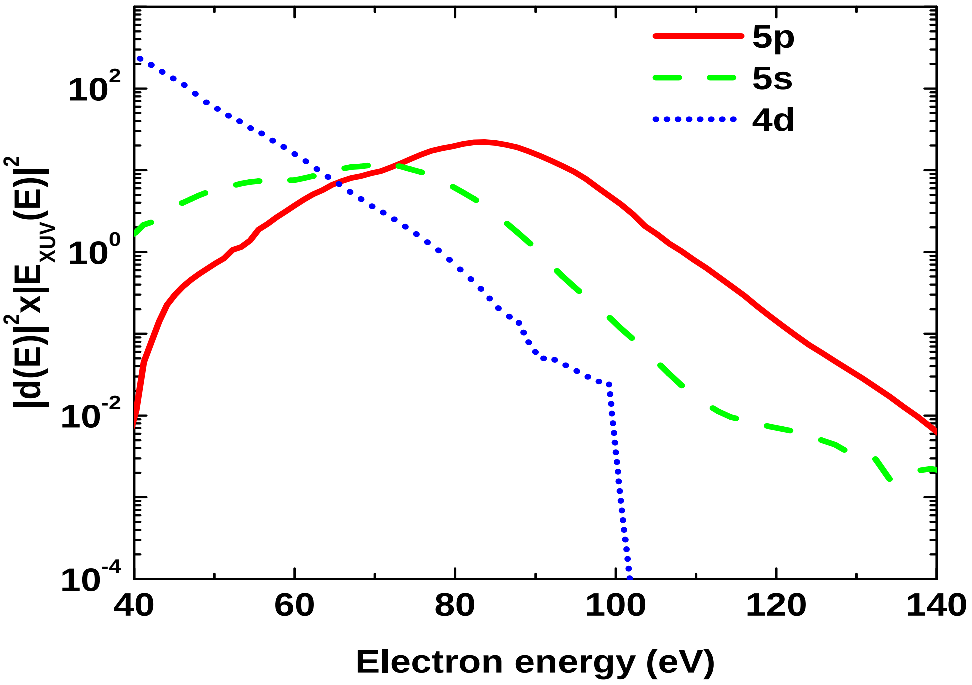


FIG. S2: (Color online) Contributions of photoelectrons from different subshells to the ionization of Xe by the SXR in the experiment of Ref.[1]. The photon energy is expressed as E+$I_P$ for each subshell. The sharp cutoff near 100 eV for 4d shell is due to the spectral range of the SXR pulse.

traces and ACs using the SXR phases and vector potential of the MIR retrieved from the PROBP-AC method.

Table S1 summarizes the merits for the retrieval of experimental data based on our PROBP-AC method and with the retrieved pulse using ML-VTGPA from Ref.[1]. We use 40 × 40 grid points for the AC in the region of $\tau_1 \in [-4 \text{ fs}, 0 \text{ fs}]$ and $\tau_2 \in [-8 \text{ fs}, -4 \text{ fs}]$ for the retrieval and merit calculations. More points are used for comparison of the streaking traces. A total of 200 grid points in time delay axis (−10 fs to 10 fs) and 320 grid points in energy axis (40 eV to 140 eV) are used. Table S1 shows that the merit using PROBP-AC method including 5p, 5s and 4d channels give the best merits, using both the streaking spectrogram or the AC pattern. If the contribution of photoelectrons from 4d is not included, i.e., only including 5s and 5p, then the merits increase slightly, meaning that the retrieval is not as good as the one including all three channels. This is consistent with the results in Fig. S3. On the other hand, the merits calculated using the experimental and the retrieved spectrograms provided from Ref.[1] show significantly larger merits, for both calculated from the streaking traces or from the AC patterns. Based on the comparison of the AC patterns in Fig. 3 of the main text and the merits shown in Table S1, we believe it is fair to claim that the SXR pulses retrieved from this work is more accurate.

Similarly, we compare the merits using the experimental data of Ref.[2]. We use 121 × 121 grid points for the AC in the region of $\tau_1 \in [-2 \text{ fs}, 4 \text{ fs}]$ and $\tau_2 \in [-2 \text{ fs}, 4 \text{ fs}]$. A total number of 160 grid points in time delay axis (−4 fs to 4 fs) and 40 grid points in energy axis (50 eV to 350 eV) are used for the streaking traces. The results are shown in Table S2. Note that the retrieved spectrogram used for the analysis was generated by us using the pulse parameters reported in Ref.[2]. From Table S2, we note that in both cases, the PROBP-AC method gives smaller values for the merit, thus demonstrating that the SXR pulses are more accurately retrieved using the PROBP-AC method than reported in the original paper.

| | $\varepsilon_S$ | $\varepsilon_{AC}$ |
|---|---|---|
| PROBP-AC (with $5p + 5s$ ) | 0.012 | 0.042 |
| PROBP-AC (with $5p + 5s + 4d$) | 0.010 | 0.030 |
| ML-VTGPA (with $5p + 5s$ ) | 0.019 | 0.090 |

TABLE S1: Merits of the streaking traces ($\varepsilon_S$) and the AC patterns ($\varepsilon_{AC}$)for the experimental data of [1] obtained using different retrieval methods. The merit from ML-VTGPA is obtained from the spectrogram retrieved in [1].

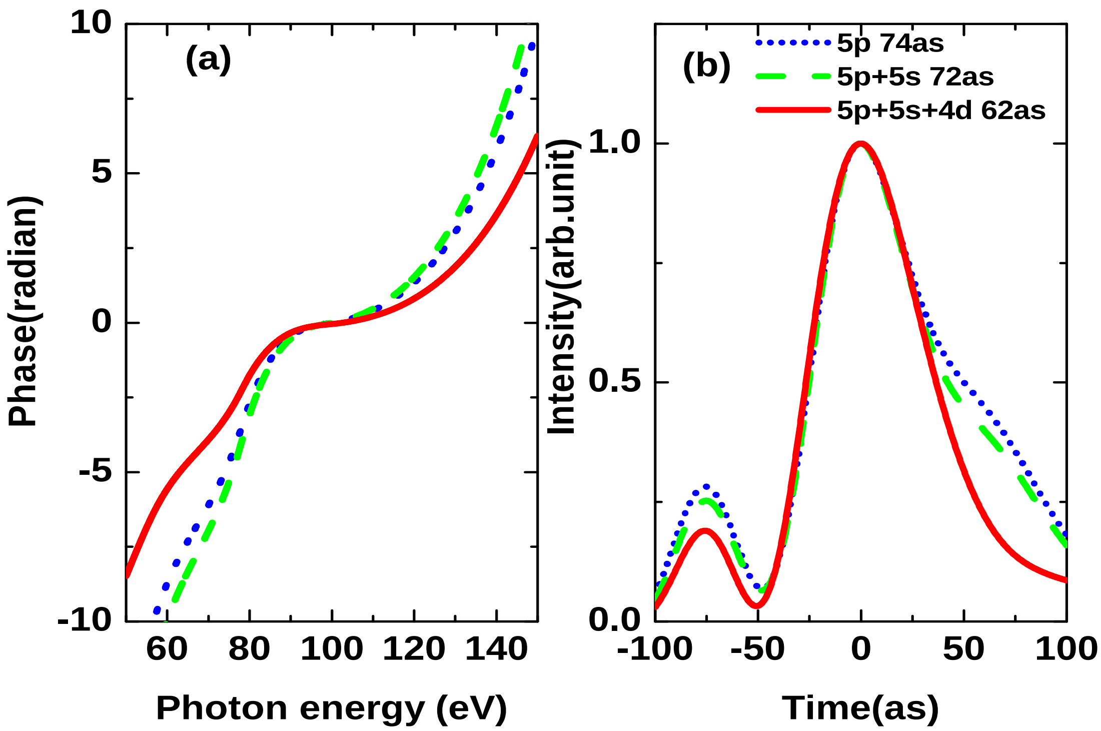


FIG. S3: (Color online) (a) Retrieved spectral phases with inclusion of $5p$ channel only (red solid), $5p + 5s$ channels (green dashed), and all three $5p + 5s + 4d$ channels (blue dotted). (b) The corresponding retrieved temporal intensity envelopes, respectively.

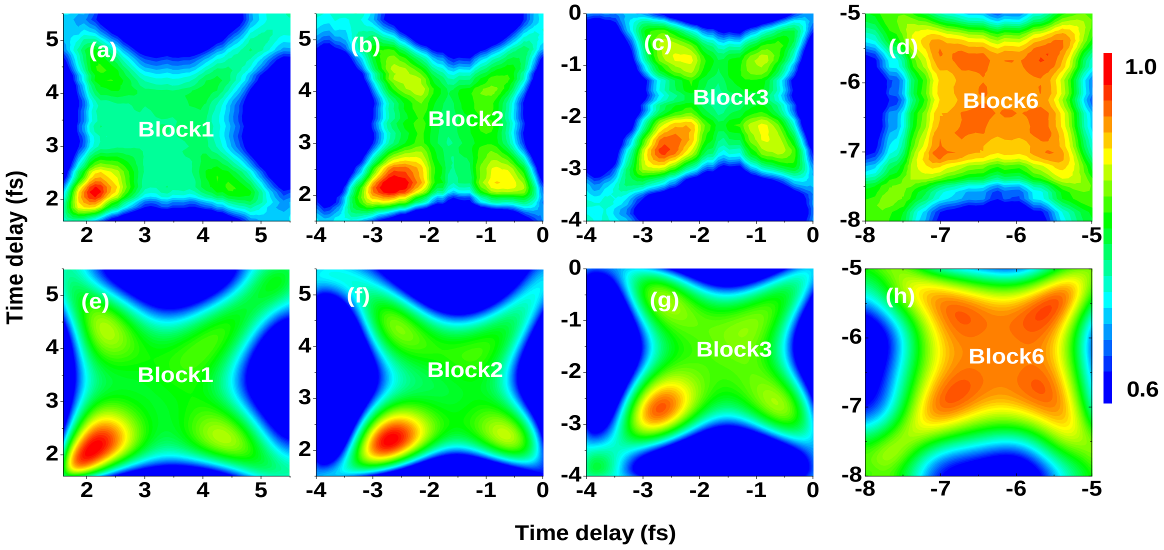


FIG. S4: (Color online) Experimental AC patterns (a-d) and their corresponding AC patterns (e-f) retrieved using the PROBP-AC method for the four blocks indicated. Good agreement has been achieved in each case.

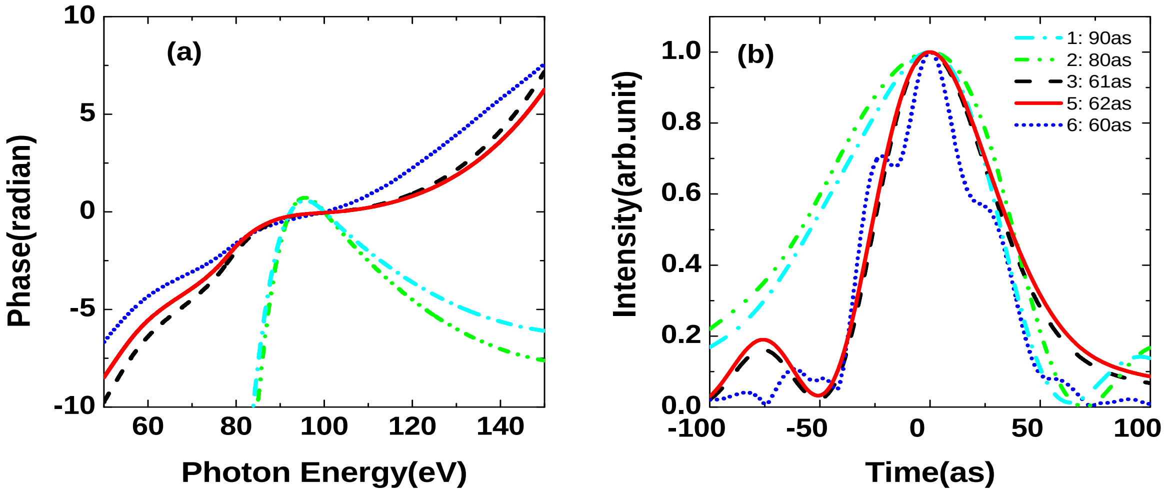


FIG. S5: (Color online) Retrieved spectral phases (a) and the temporal intensity envelopes for for Block 1,2, 3, 5 and 6, respectively.

| | $\varepsilon_S$ | $\varepsilon_{\mathrm{AC}}$ |
|---|---|---|
| PROBP-AC | 0.012 | 0.036 |
| PROOF | 0.032 | 0.061 |

TABLE S2: Merits of the streaking traces ($\varepsilon_S$) and the AC patterns ($\varepsilon_{\mathrm{AC}}$) for the experimental data of [2]. To obtain the merits for the PROOF method, we generated the spectrogram based on the published pulse parameters in the cited paper, and the MIR laser is assumed to be monochromatic as in the PROOF model.

[1] Gaumnitz, T., Jain, A., Pertot, Y., Huppert, M., Jordan, I., Lamas F. A. & Wörner, H. J. Streaking of 43-attosecond soft-X-ray pulses generated by a passively CEP-stable mid-infrared driver. Opt. Exp. **25**, 27506-27518 (2017).

[2] Li, J. *et al.* 53-attosecond X-ray pulses reach the carbon K-edge. Nat. Commun. **8** 186 (2017).
